# Supplementary material for: Network motifs emerge from interconnections that favor stability
Source: arXiv:1411.5412 source file (2014-11-20)
Supplement: Supplementary file 1 [file Motif-supplement.pdf]

# (SUPPLEMENTARY INFORMATION)
# NETWORK MOTIFS EMERGE FROM INTERCONNECTIONS THAT FAVOR STABILITY

MARCO TULIO ANGULO[1], YANG-YU LIU[2], AND JEAN-JACQUES SLOTINE[3]

1. Theoretical details 1
1.1. Preliminaries. 1
1.2. Interconnection of nodes and the optimal matrix measure. 2
1.3. Interconnection of modules. 3
2. Mean contraction loss for 3 or 4 node networks 4
3. Contraction loss with a uniform metric 5
4. Motif search and network condensation 6
5. Contraction loss of electronic circuits 7
6. Description of the network datasets 7
References 7

Contents

This supplement details the theoretical results used in the main paper and presents additional supporting material. The derivation of the theoretical results used in the paper is presented in Section 1. The detailed description of the method to compute the mean contraction loss of all subgraphs with 3 or 4 edges is presented in Section 2. The contraction loss with a uniform metric is analyzed in Section 3. The procedure used to search and condense motifs in real networks is described in Section 4. Section 5 contains a brief description of the network dataset analyzed in this work.

## 1. Theoretical details

### 1.1. Preliminaries.

**Notation.** We use $P \succ 0$ to denote a positive definite matrix, i.e., it satisfies $x^\top P x > 0$ for all $x \in \mathbb{R}^N \setminus \{0\}$. Similarly, $P \geq 0$ denotes a positive semi-definite matrix: $x^\top P x \geq 0$ for all $x \in \mathbb{R}^N \setminus \{0\}$. A matrix $Q$ is negative semi-definite if $-Q$ is positive semi-definite and we write it as $Q \leq 0$. We use $\{\lambda_i(A)\}_{i=1}^N$ to denote the set of eigenvalues of the matrix $A \in \mathbb{R}^{N\times N}$, and $\lambda_{\mathsf{max}}(A)$ to denote its eigenvalue with maximum magnitude.

The main text has used the fact that any vector norm $|\cdot|$ induces a matrix norm $\|\cdot\|$ and a matrix measure $\mu$ as

$$\|A\| \coloneqq \sup_{|x|=1} |Ax|, \quad \mu(A) \coloneqq \lim_{h \searrow 0} \frac{\|I + hA\| - 1}{h},$$

both well defined for any matrix $A \in \mathbb{R}^{N\times N}$. By using the Euclidean vector norm $|\cdot|_2$, one obtains the matrix measure

$$\mu_2(A) = \tfrac{1}{2}\lambda_{\mathsf{max}}(A + A^\top).$$

A straightforward generalization is to use of a weighted Euclidean norm $x \mapsto |Px|_2$ for some nonsingular metric $P \in \mathbb{R}^{N\times N}$ which induces the matrix measure $\mu_{2,P}(A) = \mu_2(PAP^{-1})$.

[1]Center for Complex Network Research, Northeastern University. [2]Brigham and Women's Hospital and Harvard Medical School. [3]Nonlinear Systems Laboratory, MIT. Boston, MA.

In the following theorem we show that, given a matrix $A$, the metric $P$ minimizing its matrix measure is characterized by the solution to a Linear Matrix Inequality (LMI) [1].

**Theorem 1.** *Denote by $\mathcal{M}$ the set of all matrix measures on $\mathbb{R}^{N\times N}$, then for any matrix $A \in \mathbb{R}^{N\times N}$ it holds*

$$\mu_A(A) \coloneqq \max_{1\le i\le N} \mathrm{Re}\lambda_i(A) = \min_{\mu\in\mathcal{M}} \mu(A).$$

*In addition $\mu_A = \mu_{2,P^{1/2}}$, where the metric $P = P^\top > 0$ is a solution to the linear matrix inequality $A^\top P + PA - 2\mu_A(A)P \le 0$.*

*Proof.* It is known (see e.g. [2]) that any matrix measure $\mu$ satisfies $\max_i \mathrm{Re}\lambda_i(A) \le \mu(A)$. It is also known (see Lemma 2 from [3]) that if for some $P = P^\top > 0$, $A^\top P + PA - 2\mu P \le 0$, then $\mu_{2,P^{1/2}}(A) \le \mu$.

Then the theorem will be proven if we can show that there exists $P = P^\top > 0$ solution to $A^\top P + PA - 2\mu_A(A)P \le 0$, since in such case we have $\mu_A(A) = \max_i \mathrm{Re}\lambda_i(A) \le \mu_{2,P^{1/2}}(A)$ and also $\mu_{2,P^{1/2}}(A) \le \mu_A(A)$, that together imply that $\mu_{2,P^{1/2}}(A) = \mu_A(A)$.

One can rewrite $A^\top P + PA - 2\mu_A(A)P \le 0$ as $[A^\top - \max_i \mathrm{Re}\lambda_i(A)I]P + P[A - \max_i \mathrm{Re}\lambda_i(A)I] \le 0$ with $I \in \mathbb{R}^{N\times N}$ the identity matrix. The matrix $A - \max_i \mathrm{Re}\lambda_i(A)I$ is stable (although not necessarily asymptotically-stable), since its eigenvalues have non-positive real part. Therefore, there exists a symmetric positive definite solution $P$ to $[A^\top - \max_i \mathrm{Re}\lambda_i(A)I]P + P[A - \max_i \mathrm{Re}\lambda_i(A)I] \le 0$, completing the proof of the Theorem. □

The solution $P$ to the LMI in Theorem 1 can be easily computed using MATLAB with CVX [4] and the following code:

```
n=length(A);
mu= max(real(eig(A)));
cvx_begin sdp
        variable P(n,n) symmetric semidefinite
        A'*P + P*A - 2*mu*P<= 0
        P >= (1e-5)*eye(n)
cvx_end
```

When the matrix $A$ is Metzler, there always exists a diagonal solution $P$ to the LMI in Theorem 1, see Proposition 1 of [5]. This implies that the metric reduces to a particular choice of units for each node.

## 1.2. Interconnection of nodes and the optimal matrix measure.

In the main text, we started by considering the interconnection of $N$ scalar nodes

$$\text{(1)} \qquad \begin{cases} \dot{x}_i = f_i(x_i,t) + u_i \\ y_i = x_i \end{cases} \qquad x_i(t_0) = x_{i0}, \quad i = 1,\cdots,N,$$

where the scalars $x_i$, $u_i$ and $y_i$ are the state, input and output of node $i$, respectively. Each node is assumed to be contracting with rate $\alpha_i > 0$. Nodes interact with each other by interconnecting their inputs and outputs as follows

$$\text{(2)} \qquad u = Ay,$$

where $y = \mathrm{col}(y_1,\cdots,y_N)$, $u = \mathrm{col}(u_1,\cdots,u_N)$ and $A \in \mathbb{R}^{N\times N}$ is the weighted adjacency matrix of the interconnection network.

Denoting by $J(x,t)$ the Jacobian of the network system (1)-(2), the interconnected system remains contracting if there exists a matrix measure $\mu \in \mathcal{M}$ such that

$$\mu\big(J(x,t)\big) \leq \mu(-D_\alpha) + \mu(A) < 0$$

where $D_\alpha = \mathsf{diag}\{\alpha_1, \cdots, \alpha_N\}$. We further defined $\mu(A)$ as the contraction loss of the interconnection network, and asked for the optimal choice of matrix measure for which the left hand side of the inequality above is as negative as possible.

The following proposition characterizes the optimal matrix measure in the case when $A$ is Metzler.

**Proposition 1.** *If the off-diagonal entries of $A$ are non-negative (i.e. $A$ is Metzler), then $\mu_A$ is the optimal choice of matrix measure.*

*Proof.* From Theorem 1 the optimal matrix measure for any matrix $A$ is $\mu_A$, with associated optimal metric $P$. Since $A$ is assumed Metzler, $P$ is diagonal and $\mu_A$ is also the optimal matrix measure for $-D_\alpha$ since

$$\mu_A(-D_\alpha) = \mu_2(-P^{1/2} D_\alpha P^{-1/2}) = \mu_2(-D_\alpha) = -\alpha_{\mathsf{min}}$$

and $\mu_{-D_\alpha}(-D_\alpha) = -\alpha_{\mathsf{min}}$ is the optimal matrix measure for $-D_\alpha$. Above $\alpha_{\mathsf{min}} = \mathsf{min}\{\alpha_1, \cdots, \alpha_N\}$ is the minimal contraction rate of the isolated nodes and we have used the fact that $P^{1/2} D_\alpha P^{-1/2} = D_\alpha$ since $P$ and $D_\alpha$ are diagonal matrices. □

In the case when $A$ is not Metzler, it is convenient to consider an identical contraction rate for all isolated nodes. Namely, if each isolated node is contracting with rate $\alpha_i$, then it is also contracting with a smaller rate $\alpha_{\mathsf{min}}$. Using this underestimation yields $D_\alpha = -\alpha_{\mathsf{min}} I$ and we recover $\mu_A(-D_\alpha) = -\alpha_{\mathsf{min}}$.

### 1.3. Interconnection of modules.

In the second part of the main text we consider the interconnection of $N$ modules possibly having vector dynamics

(3)
$$\begin{cases} \dot{x}_i = f_i(x_i, t) + B_i u_i \\ y_i = C_i x_i \end{cases} \qquad x_i(t_0) = x_{i0}, \;\; i = 1, \cdots, N,$$

where $x_i \in \mathbb{R}^{n_i}$, $u_i \in \mathbb{R}^{m_i}$ and $y_i \in \mathbb{R}^{p_i}$ are the state, input and output vectors of module $i$. The interconnection of modules is again described by equation (2), but the $A$ matrix is not square anymore if some module has different number of inputs and outputs. We assumed no self-loop in the interconnection of modules.

Each isolated module was assumed contracting with rate $\alpha_i > 0$ and measure $\mu_i$, and we associated a condensed scalar node inheriting the module's contraction rate

(4)
$$\begin{cases} \dot{z}_i = -\alpha_i z_i + u_i \\ y_i = z_i \end{cases} \qquad i = 1, \cdots, N.$$

Additionally, we defined the condensed adjacency matrix $A_{\mathsf{cond}} \in \mathbb{R}^{N \times N}$ as

(5)
$$A_{\mathsf{cond}} \coloneqq \begin{bmatrix} 0 & \|M_{12}\|_{1,2} & \cdots & \|M_{1N}\|_{1,N} \\ \|M_{21}\|_{2,1} & 0 & \cdots & \|M_{2N}\|_{2,N} \\ \vdots & & \ddots & \vdots \\ \|M_{N1}\|_{N,1} & \|M_{N2}\|_{N,2} & \cdots & 0 \end{bmatrix},$$

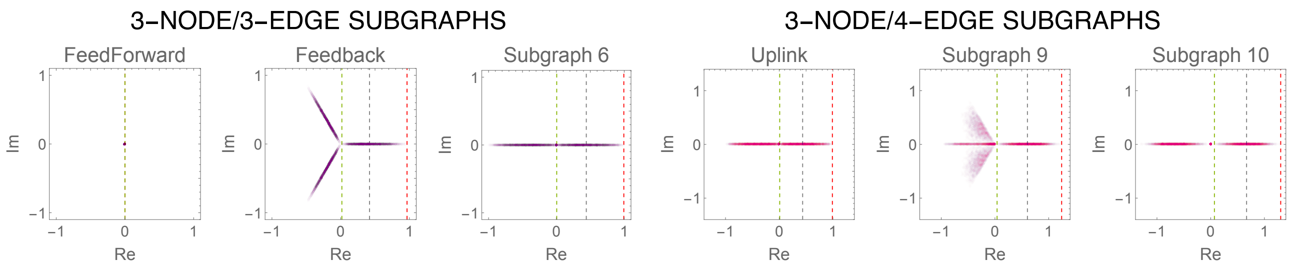


FIGURE S1. Mean contraction loss using the matrix measure $\mu_A$ for different 3-node subgraphs. For each interconnection $A$, we generate 10,000 matrices with the same interconnection pattern and uniform weights between $[0,1]$ and plot their corresponding eigenvalues in the complex plane. The mean contraction loss of $A$ corresponds to the average of the largest eigenvalue, marked with a dashed black line. Maximum and minimum values for the contraction loss are also marked in red and green dashed lines, respectively.

where $M_{ij} = B_i A_{ij} C_j$ with $A_{ij}$ the $(i,j)$ block of the original interconnection network (2). Above $\|\cdot\|_{i,j}$ stands for the induced matrix norm

$$\|M\|_{i,j} \coloneqq \sup_{|x|_i=1} |Mx|_j$$

with $|x|_i = |P_i^{1/2} x|_2$ a weighted Euclidean norm with metric $P_i \in \mathbb{R}^{n_i \times n_i}$ found as the solution to LMI in Theorem 1.

Then we used the following theorem to prove the contraction of the original network by means of a condensed network.

**Theorem 2.** *If the condensed interconnected system (4)-(5) is contracting, then the original interconnected system (3)-(2) is also contracting.*

*Proof.* Each isolated module is assuming contracting with rate $\alpha_i$ and matrix measure $\mu_i$, i.e. $\mu_i(J_i(x_i,t)) \le -\alpha_i$, $\forall x, \forall t \ge t_0$. Define $B = \mathsf{blockdiag}\{B_1, \cdots, B_N\}$ and $C = \mathsf{blockdiag}\{C_1, \cdots, C_N\}$. The Jacobian of the original interconnected system is

$$J(x,t) = \mathsf{blockdiag}\{J_1, \cdots, J_N\} + BAC$$

where $J_i = J_i(x_i,t)$ is the Jacobian of the $i$-th isolated module. Define the "structural" Jacobian as

$$J_{\mathsf{S}}(x,t) = \mathsf{blockdiag}\{\mu_1(J_1), \cdots, \mu_N(J_N)\} + A_{\mathsf{cond}}$$

Theorem 2 in [6] proves that $\mu(J) \le \mu(J_{\mathsf{S}})$. Finally, noticing that $\mu(J_{\mathsf{S}}) \le \mu(-D_\alpha) + \mu(A_{\mathsf{cond}})$ completes the proof. □

## 2. Mean contraction loss for 3 or 4 node networks

We start with two lists, the first containing all subgraphs with three nodes ($2^9 = 512$ in total) and the second all networks with four nodes ($2^{16} = 65536$ in total). By removing from the lists all subgraphs that are isomorphic or that have self-loops, we obtain 13 three-node subgraphs and 199 four-node subgraphs.

For each subgraph in each list we can compute its adjacency matrix $A$, which is a binary matrix containing only the interconnection pattern of the system. In contrast, a network coming from a dynamic model (for example from a linearization of a nonlinear system) usually contains real coefficients representing the strength of the interaction between nodes. To circumvent this problem, we compute

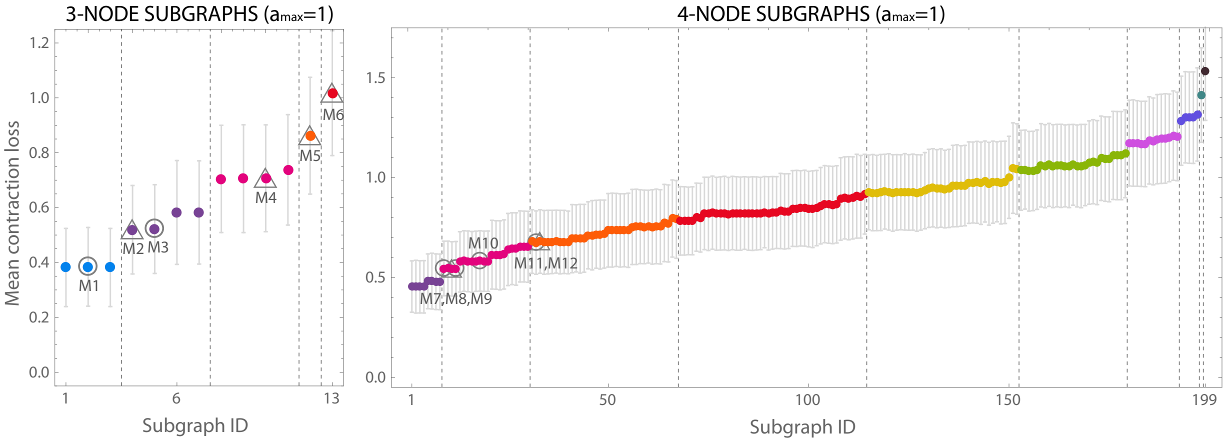


FIGURE S2. Mean contraction loss of all subgraphs with 3 and 4 nodes using a uniform metric (i.e. the matrix measure $\mu_2$). Same color indicates same number of edges. Vertical dashed lines separate groups of subgraphs with the same number of edges (density classes) in increasing order from left to right (2 to 6 edges for 3-node subgraphs, and 3 to 12 edges for 4-node subgraphs). Gray marks show the network motifs found in [7], circles denoting biological related networks (gene transcription, neurons and food webs) and triangles man-made networks (electronic circuits and the WWW).

the *mean* contraction loss from an ensemble of matrices with the same interconnection pattern but with random positive entries.

More precisely, we define the mean contraction loss $\langle\mu\rangle$ of a binary matrix $A$ as

$$\langle \mu(A) \rangle = \lim_{k\to\infty} \frac{1}{k} \sum_{i=1}^{k} \mu(A_i),$$

where the matrices $\{A_i\}_{i=1}^{k}$ are constructed with the same pattern of zeros as $A$, but with nonzero entries randomly (and independently) chosen from a uniform distribution with support in $[0, a_{\mathsf{max}}]$ for some $a_{\mathsf{max}} > 0$. The value of $a_{\mathsf{max}}$ just scales the mean contraction loss, since matrix measures are positive homogeneous $\mu(a_{\mathsf{max}}A) = a_{\mathsf{max}}\mu(A)$ for any $a_{\mathsf{max}} \geq 0$, [2]. In the paper, we approximate the limit by taking the mean of $k = 10\,000$ terms. In Figure S1 we illustrate the process in a more intuitive way.

## 3. Contraction loss with a uniform metric

In the main text, we have used the optimal matrix measure $\mu_A$ to compute the contraction loss of an interconnection network $A$. We have seen that this corresponds to introducing different metrics $P_i$ to different modules in the network. Different metrics make more complicated the interconnection between modules, since each module needs to know the particular metric of all other modules to which it is connected to compute the induced matrix norms that appear in $A_{\mathsf{cond}}$. Thus, nature may prefer to use the same metric for all modules to avoid this.

By using a uniform metric for all modules, one may assume that all matrices $A \in \mathbb{R}^{N\times N}$ are equally probable to appear, so there is no possible preference in the metric to use. This suggest to use the identity metric $P = I$ which induces the simple Euclidean matrix measure $\mu_2$.

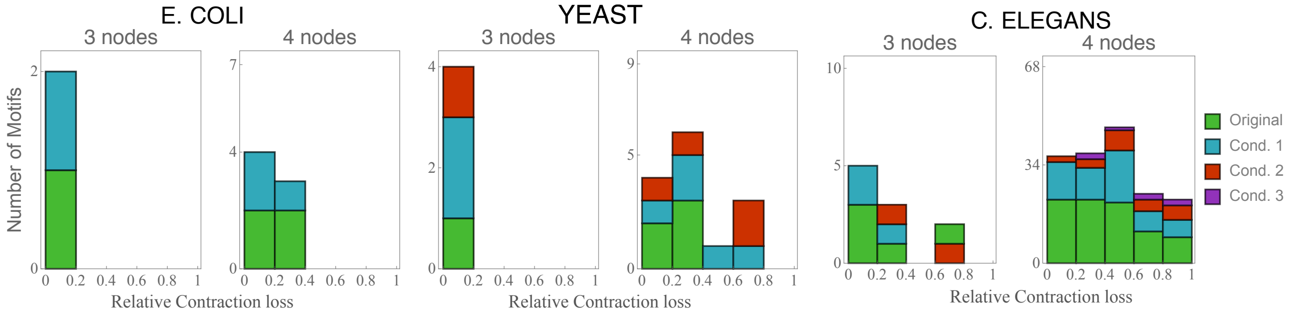


FIGURE S3. Number of motifs vs relative contraction loss using the matrix measure $\mu_2$. Original and condensed networks are shown in different colors. The Saint Martin food-web network is not shown since it does not contain motifs after a single condensation.

With the matrix measure $\mu_2$, we compute the mean contraction loss of all 3 and 4 node subgraphs, obtaining the results shown in Figure S2. Compared to the results obtained using the optimal matrix measure $\mu_A$, we observe that the difference in contraction loss among subgraphs in the same density class is smaller and there is no subgraph with zero contraction loss. However, we observe that only Motif 10 in Figure 1 of the main paper fails to have the lowest mean contraction loss in its density class. This means that 11 of 12 motifs have low relative contraction loss with the uniform metric, compared to 9 of 12 using the optimal metric.

In contrast with the optimal metric, the uniform metric shows that most 4-node motifs have low relative contraction loss in the original and condensed C. Elegans networks, see Figure S3.

## 4. Motif search and network condensation

Network motifs of 3 and 4 nodes were found using the mfinder program[1]. We run the program using the following options

```
./mfinder <network.dat> − s N − r 1000 −omem −maxmem 5000000
```

where network.dat is the file with the edgelist of the network and N is the motif-size to search (N= 3 or 4). The output of the program is a text file network_OUT.txt which contains a report of the motifs found, together with the $Z$-score, $P$-value and uniqueness of each subgraph of size N in the network. With the used options, mfinder also generates a text file network_MEMBERS.txt containing the list of all subgraphs found in the network.

Once all motifs of size 3 and 4 in the network are obtained, their corresponding subgraphs are condensed. The condensation consist in replacing all nodes in a motif by a single "condensed" node, keeping all the interconnections of the original nodes (and removing the repeated edges). If two motifs share one or more nodes, one of the two motifs is discarded at random.

The process of motif search and condensation is recursively repeated until no motif is found. The obtained results for the selection of real networks shown in Table 1.

[1] http://wws.weizmann.ac.il/mcb/UriAlon/download/network-motif-software

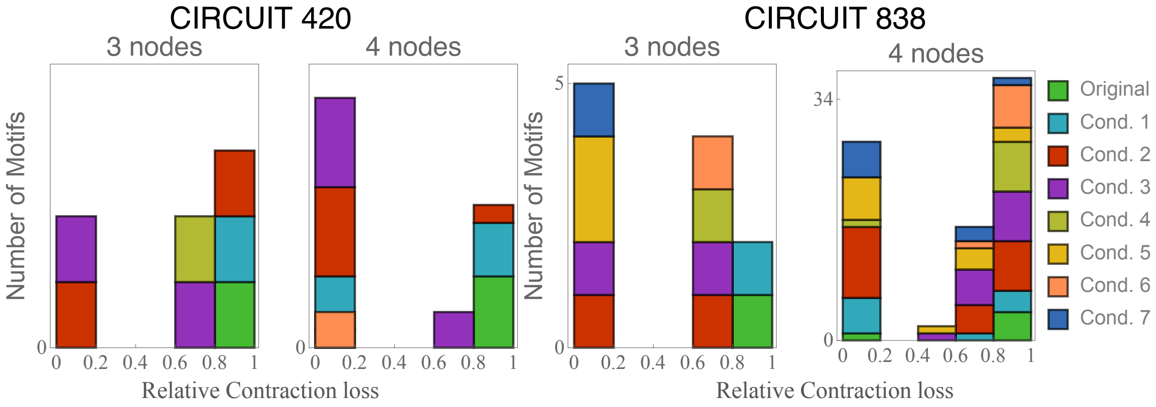


FIGURE S4. Electronic circuits. Number of motifs with low, low-medium, medium, medium-high and high relative contraction loss using the optimal matrix measure $\mu_A$. Original and condensed networks are shown in different colors.

## 5. Contraction loss of electronic circuits

Here we present the analysis of the contraction loss of 3- and 4-node motifs for two electronic circuits. In contrast to the network considered in the main text, these ones are man-made and contain feedback motifs with high $Z$-score.

Compared to biological networks, we find that these networks can be condensed more times. The histograms counting the number of motifs at a given bin of relative contraction loss is presented in Figure S4. In contrast to biological networks, we find that most motifs in the original and condensed networks have high relative contraction loss.

## 6. Description of the network datasets

Following [8], network are pre-processed by removing mutual edges if they constitute less that 0.1% of the edges of the network. In this process, only one edge from the Yeast network is removed.

| NETWORK NAME | $N$ | $E$ | DESCRIPTION |
|---|---|---|---|
| C. Elegans [9] | 297 | 2 345 | Neural network of C. Elegans |
| E. Coli [7] | 418 | 519 | Transcription regulatory network of E. Coli |
| Yeast [7] | 688 | 1 079 | Transcription regulatory network of S. Cerevisiae |
| Saint Martin [7] | 688 | 1 079 | Food Web in Saint Martin |
| Circuit 420 [7] | 252 | 399 | Digital fractional multiplier |
| Circuit 838 [7] | 512 | 819 | Digital fractional multiplier |

TABLE 1. Real networks used in our study. For each network we show its number of nodes ($N$) and edges ($E$), together with a brief description.

## References

[1] S. P. Boyd, L. El Ghaoui, E. Feron, and V. Balakrishnan, *Linear matrix inequalities in system and control theory*. SIAM, 1994, vol. 15.

[2] C. Desoer and H. Haneda, "The measure of a matrix as a tool to analyze computer algorithms for circuit analysis," *Circuit Theory, IEEE Transactions on*, vol. 19, no. 5, pp. 480–486, 1972.

[3] Z. Aminzare, Y. Shafi, M. Arcak, and E. D. Sontag, "Guaranteeing spatial uniformity in reaction-diffusion systems using weighted lˆ 2 norm contractions," in *A Systems Theoretic Approach to Systems and Synthetic Biology I: Models and System Characterizations*. Springer, 2014, pp. 73–101.

[4] M. Grant and S. Boyd, "CVX: Matlab software for disciplined convex programming, version 2.1," http://cvxr.com/cvx, Mar. 2014.

[5] A. Rantzer, "Distributed control of positive systems," *CoRR*, vol. abs/1203.0047, 2012.

[6] G. Russo, M. di Bernardo, and E. Sontag, "A contraction approach to the hierarchical analysis and design of networked systems," *Automatic Control, IEEE Transactions on*, vol. 58, no. 5, pp. 1328–1331, May 2013.

[7] R. Milo, S. Shen-Orr, S. Itzkovitz, N. Kashtan, D. Chklovskii, and U. Alon, "Network motifs: simple building blocks of complex networks," *Science*, vol. 298, no. 5594, pp. 824–827, 2002.

[8] R. Milo, S. Itzkovitz, N. Kashtan, R. Levitt, S. Shen-Orr, I. Ayzenshtat, M. Sheffer, and U. Alon, "Superfamilies of evolved and designed networks," *Science*, vol. 303, no. 5663, pp. 1538–1542, 2004.

[9] D. J. Watts and S. H. Strogatz, "Collective dynamics of ?small-world?networks," *nature*, vol. 393, no. 6684, pp. 440–442, 1998.
